# Supplementary material for: MaPa: Text-driven Photorealistic Material Painting for 3D Shapes
Source: arXiv:2404.17569 source file (2026-10-01)
Supplement: Supplementary file 1 [file 06_supp.tex]

\section{Implementation details of segment-conditioned ControlNet}
% 我们的segment-controlled ControlNet的输入是一个segmentation mask。
% The 2D segments are sorted by area size and numbered from large to small to form the 2D segmentation mask.
% 背景为0.
Our segment-controlled ControlNet takes a segmentation mask as input.
The 2D segments are sorted by area size and numbered from large to small to form the 2D segmentation mask, and the background is set to 0.
Our segment-controlled ControlNet is implemented based on the SAM-conditioned ControlNet~\cite{gao2023editanything}. 
We find the original SAM-conditioned ControlNet is not suitable for our task, because it tends to fail in object-centric image generation. 
% 如果有大面积的segmentation mask被标注为0的话。
It may generate noisy images, if there are large areas of the segmentation mask are labeled as 0.
We finetune the SAM-conditioned ControlNet on our dataset to make it more suitable for our input.
We collect about 10K 3D models from Objaverse-LVIS~\cite{deitke2023objaverse} dataset and label each 3D model with textual descriptions using BLIP~\cite{li2022blip}.
To generate corresponding images with paired segmentation masks for finetuning the SAM-conditioned ControlNet, we render each object 
into 16 depth maps with random sampled viewpoints to generate RGB images with Depth-to-image diffusion~\cite{rombach2022high} and segment them by SAM~\cite{kirillov2023segment} to obtain the segmentation mask.
The viewpoints are randomly sampled from a complete 360-degree horizontal angle, with vertical angles ranging from 25 to 75 degrees, and at distances varying between 1.7 and 2.3 units from the mesh. 
As we have the object mask rendered by 3D models, we can use the object mask to set the background of the segmentation mask to 0. 
%We use the depth maps to generate RGB images with Depth-to-image diffusion~\cite{rombach2022high}. Then, the images are segmented by SAM~\cite{kirillov2023segment} to obtain the segmentation mask. 

\section{The significance of segment-controlled image generation}
To evaluate the effectiveness of our segment-controlled image generation, we compare our method with the depth-to-image diffusion model which is used in TEXTure~\cite{richardson2023texture}, referred as ``D2I''.
Apart from the different diffusion model, all other modules in the baseline remain unchanged compared to our method. We select the material graph with a black uniform texture as the initial material graph to ensure fair comparison.
% 我们将这个baseline简写成d2i。
It is apparent that the depth-to-image diffusion model often produces images with appearances that mismatch the input segments. 
Since the images generated by the depth-to-image diffusion model have multiple color blocks within a segment, the texture generated by the material graph will try to match these color blocks. This leads to unstable material graph optimization and make material graph overfit the generated images.
Texture artifacts can be observed in the base color map, as shown in Figure~\ref{fig:ablation_depth}.

\input{contents/ablation_depth/ablation_depth.tex}

\section{The prompt of the material classification}
We use the GPT-4v to classify the material type.
We present an example of a visual prompt in Figure~\ref{fig:prompt}.
Our text prompt is ``You are a CG artist, and there is a material classification problem. The left image is the original image. We have created a red bounding box to highlight the region of interest, and we have cropped that region on the right image. Your task is to determine the material type of the highlighted area based on the image. If the area is too small to determine the material, please make an inference based on the surrounding information. Pay more attention to the image on the right and the surrounding area, as well as the roughness and reflectivity of the selected object. Please choose from the following material classes: [wood, metal, plastic, leather, fabric, glass, stone, ceramic, rubber]. Your answer should be in the format: output='material class'.''.

\input{contents/prompt/prompt.tex}

\section{Implementation details of Albedo estimation network}
Our albedo estimation network is implemented based on the image-conditioned stable diffusion released by Lambda Labs~\cite{huggingfaceStableDiffusion}. We finetune it on the ABO material dataset~\cite{collins2022abo}. The input image is encoded by the CLIP encoder~\cite{radford2021learning}, and then injected into the diffusion model. The diffusion model is trained to minimize the loss between the generated albedo image and ground-truth albedo image.

\section{Implementation details of material graph optimization}
% 我们的loss函数包含albedo loss和rendering loss。
Our loss function contains albedo loss and rendering loss.
The albedo loss is used to ensure that the rendered albedo image is close to the predicted albedo image.
The albedo loss function is defined as:
\begin{equation}
    \mathcal{L}_{albedo} =  \| \mu(\mathbf{A} \cdot \mathbf{M}) - \mu(\mathbf{A}^* \cdot \mathbf{M}) \|,
\end{equation}
where $\mathbf{A}$ is the rendered albedo image, $\mathbf{A}^*$ is the predicted albedo image, $\mu(\cdot)$ is the mean value of the image, and $\mathbf{M}$ is the material group mask.

The rendering loss is adopted to make the rendered image close to the generated image.
We apply masked L1 loss and masked style loss (Gram matrices of VGG features~\cite{gatys2016image}). The rendering loss function is defined as:
\begin{equation}
    \mathcal{L}_{render} = \mathcal{L}_{L1} + \mathcal{L}_{style},
\end{equation}
The final loss function is defined as:
\begin{equation}
    \mathcal{L} = \mathcal{L}_{albedo} + \mathcal{L}_{render}.
\end{equation}
% In addition, we 在优化之前会初始化uv map的stexture transform. Following PSDR-room~\cite{yan2023psdr}, we use the uv map of the input mesh as the initial uv map.
In addition, we initialize the texture transform of the uv map before optimization. Following PSDR-room~\cite{yan2023psdr}, we evaluate the selected material at various scales (ranging from 0.5 to 8.0) and orientations (-45, 0, 45, 90 degrees), aiming to identify the combination that results in the lowest Gram matrix loss between the rendered image and the generated image. We also optimize the transform of the uv map during the material graph optimization.
The number of material graphs in each category is shown in Table~\ref{tab:material_category}.

\begin{table}[t]
    \centering
    \caption{Number of material graphs in various categories.}
    \begin{tabular}{|l|c|}
    \hline
    \textbf{Material Category} & \textbf{Number of Material Graphs} \\ \hline
    Wood                       & 11                                 \\ \hline
    Metal                      & 18                                 \\ \hline
    Plastic                    & 12                                 \\ \hline
    Leather                    & 10                                 \\ \hline
    Fabric                     & 22                                 \\ \hline
    Stone                      & 5                                  \\ \hline
    Ceramic                    & 3                                  \\ \hline
    Rubber                     & 3                                  \\ \hline
    \end{tabular}

\label{tab:material_category}
\end{table}

\section{Implementation details of Downstream editing}
%这仅仅是一个有趣的application
%Note that this is just an interesting application of our method.
In this section, we describe how to implement downstream editing, which is an interesting application of our method. 
We provide GPT-4 with some APIs, allowing GPT-4 to select the appropriate API according to the user's textual instructions and generate the corresponding parameters.
Their descriptions and several in-context examples (the instructions and programs pairs) are added to GPT-4's knowledge base, when enabling it to select suitable functions and generate parameters from text instructions and information of the material graph that needs to be modified.
We also input the material type of the material graph that the user needs to edit into GPT-4, so that GPT-4 can select the appropriate API.

Additionally, we use GPT-4 to generate descriptions of geometric seamless pattern and noise texture patterns. 
The descriptions contain high-level information of the patterns, such as metaphors, feelings, emotions, semantics, and low-level information such as geometric shapes and arrangements.
These descriptions are then added into GPT-4's database, allowing GPT-4 to search for the appropriate pattern mask and noise texture pattern according to the user's textual instructions. 

Note that all the APIs and alpha mask patterns are in user's local storage.
GPT is only responsible for searching for the corresponding APIs and patterns, and generates the corresponding python commands.
Our prompt format is ``Here are the following APIs and their descriptions: \{APIs and descriptions...\}. Here are some instances demonstrating the selection of functions in response to user instructions: \{instructions and commands...\}. According to the user's instructions, you need to output the corresponding commands.''

% 我们同时将用户需要修改的material graph的material type输入到GPT-4中，以便让GPT-4选择合适的API。

Our APIs are implemented based on the filter node. Figure~\ref{fig:fx} is an example of the filter node.
We only need to add or replace the input of the filter node to add or change the texture of the material graph.
Our APIs include the following functions: add texture for fabric, change texture for fabric, add texture for ceramic, change texture for ceramic, add patinated effect for leather, add painted effect for wood, add patinated effect for wood, add patinated effect for metal, add dust, add dirt, add scratches, add water stains.
For material graphs that already have patterns, we record the nodes of each noise texture pattern that needs to be replaced.
Some filters require the user to input the color. The user can choose the default color, or input the color by themselves, or let GPT-4 recommend the color.

\begin{figure*}
\begin{center}
\setlength\tabcolsep{0.2em}
\newcommand{\mywidth}{\textwidth}
\includegraphics[width=\mywidth]{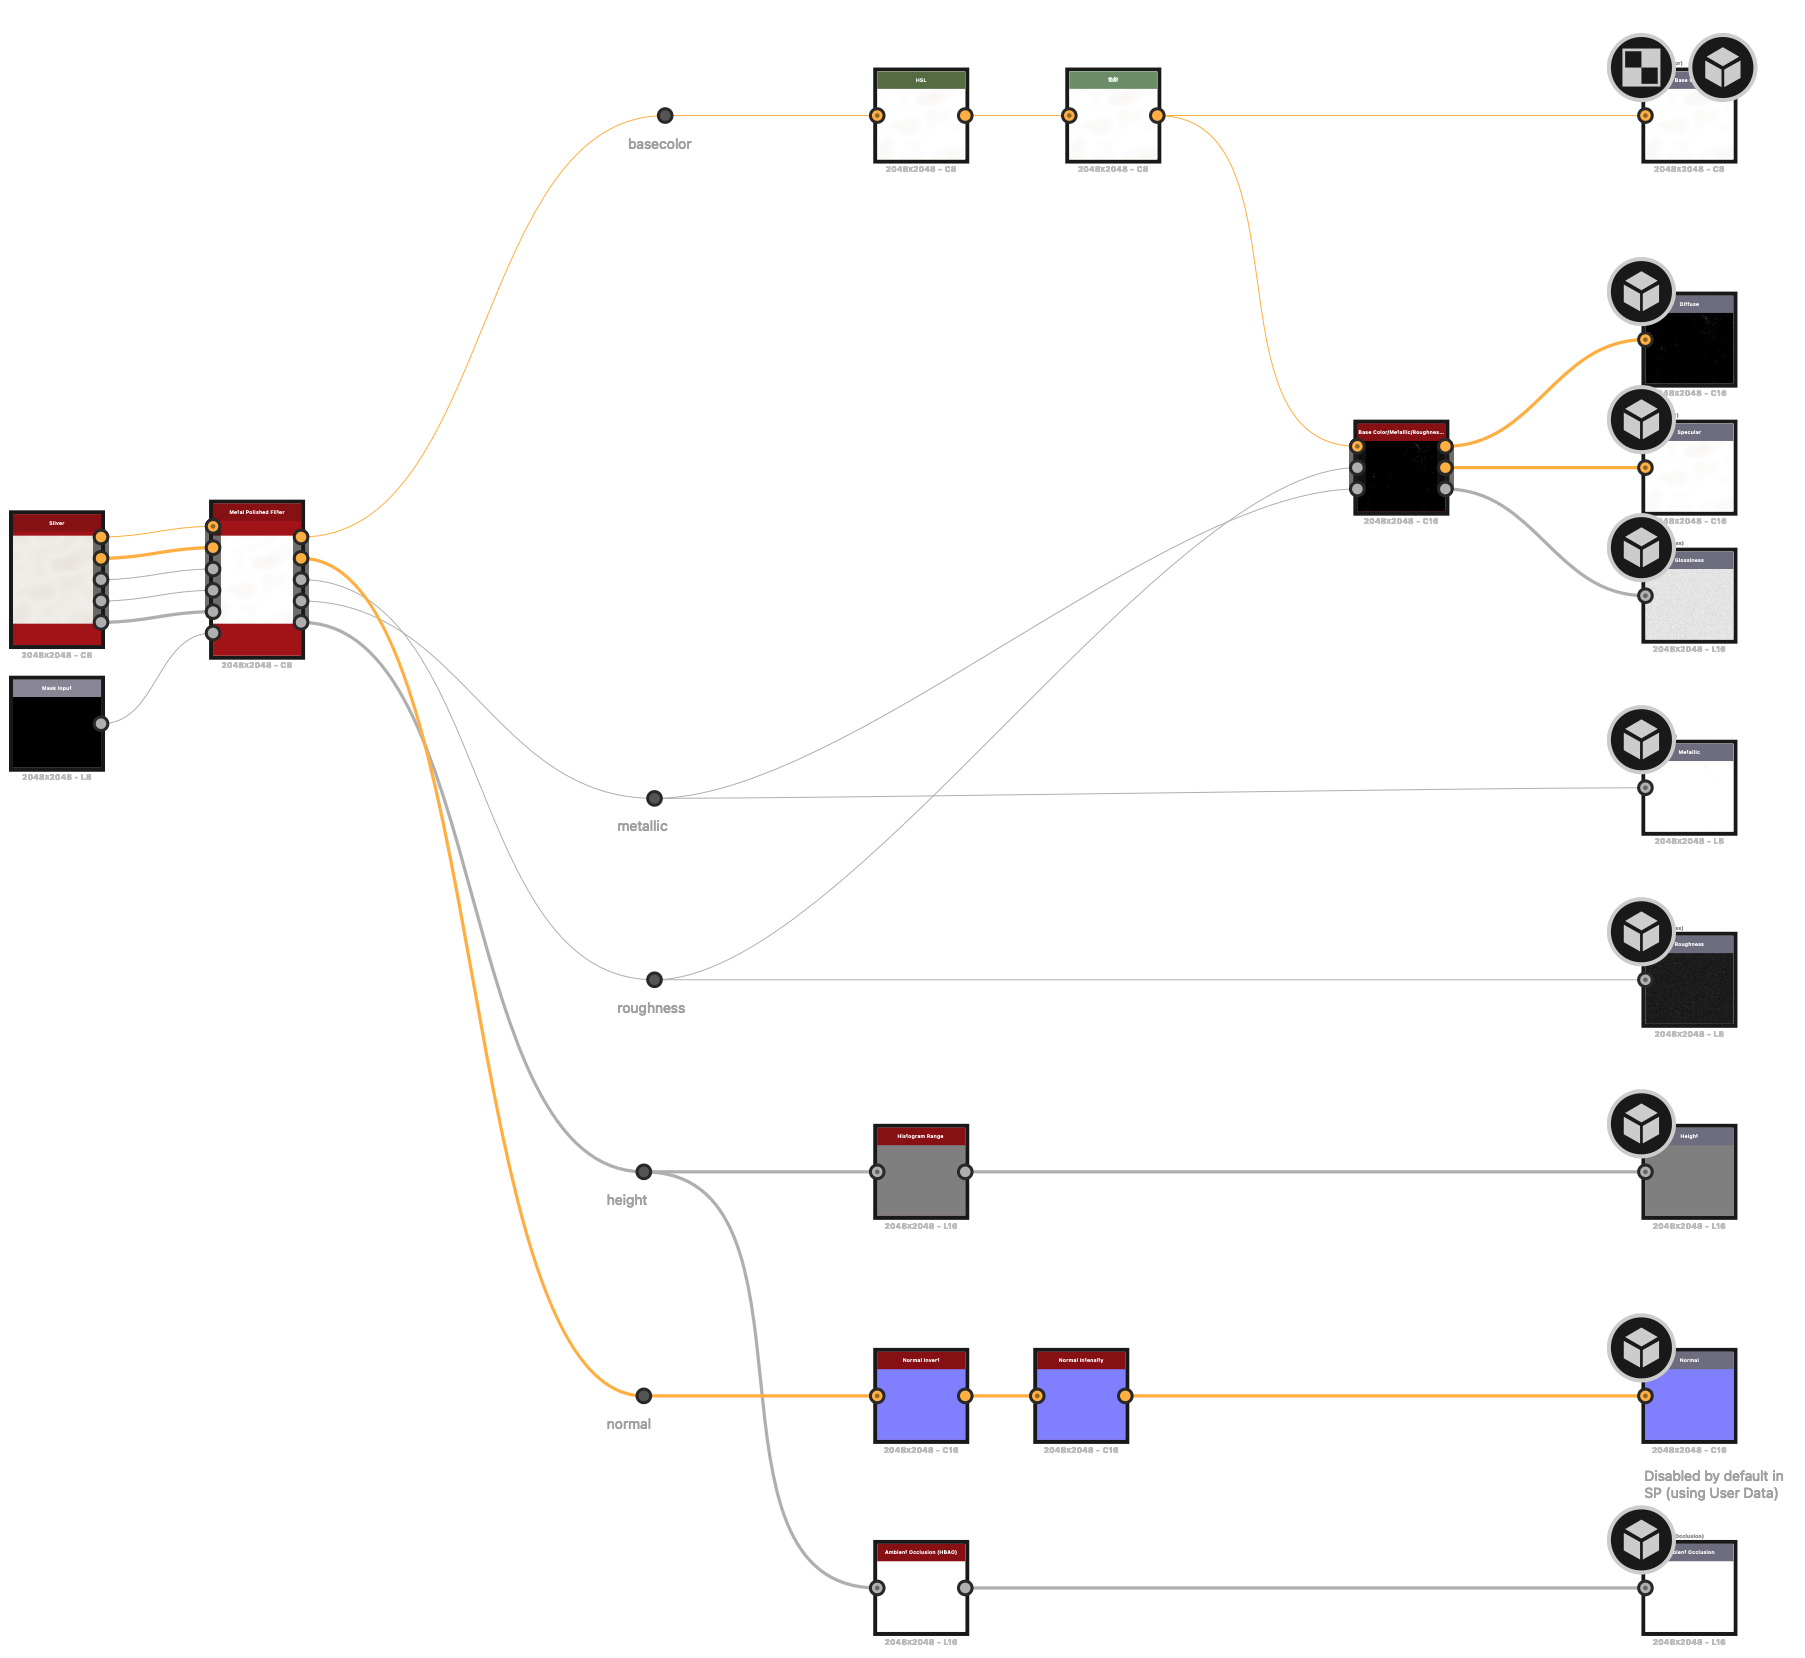}
\vspace{-1em}
\end{center}

\captionsetup{font={normalsize}} 
\caption{
\textbf{An example of the filter.} 
% 通过使用这种filter，我们可以直接替换filter input的mask和base material，输出各种各样的效果。
We can replace the mask and base material of the filter input, which can yield various results.
}
\label{fig:fx}
\end{figure*}

%\section{The number of each material category.}
